# Supplementary material for: Minimal representations of conformal groups and generalized Laguerre functions
Source: arXiv:1009.4549 source file (2012-08-27)
Supplement: Supplementary file 1 [file appendix.tex]

\chapter{Tables of simple real Jordan algebras}

\section{Structure constants}

\begin{table}
\begin{center}
\begin{tabular}[ht]{|r|c|c|c|c|c|c|c|c|c|}
  \hline
  & $V$ & $V_0$ & $n$ & $n_0$ & $r$ & $r_0$ & $d$ & $d_0$ & $e$\\
  \hline
  I$.1$ & $\Sym(n,\RR)$ & $1$ & $\frac{n}{2}(n+1)$ & $\frac{n}{2}(n+1)$ & $n$ & $n$ & $1$ & $1$ & $0$\\
  I$.2$ & $\Herm(n,\CC)$ & $2$ & $n^2$ & $n^2$ & $n$ & $n$ & $2$ & $2$ & $0$\\
  I$.3$ & $\Herm(n,\HH)$ & $3$ & $n(2n-1)$ & $n(2n-1)$ & $n$ & $n$ & $4$ & $4$ & $0$\\
  I$.4$ & $\RR^{1,n-1}$ ($n\geq3$) & $4$ & $n$ & $n$ & $2$ & $2$ & $n-2$ & $n-2$ & $0$\\
  I$.5$ & $\Herm(3,\OO)$ & $5$ & $27$ & $27$ & $3$ & $3$ & $8$ & $8$ & $0$\\
  \hline
  II$.1$ & $\times\times\times$ & $\times$ & $\times$ & $\times$ & $\times$ & $\times$ & $\times$ & $\times$ & $\times$\\
  II$.2$ & $M(n,\RR)$ & $1$ & $n^2$ & $\frac{n}{2}(n+1)$ & $n$ & $n$ & $2$ & $1$ & $0$\\
  II$.3$ & $\Skew(2n,\RR)$ & $2$ & $n(2n-1)$ & $n^2$ & $n$ & $n$ & $4$ & $2$ & $0$\\
  II$.4$ & $\RR^{p,q}$ ($p,q\geq2$) & $4$ & $p+q$ & $q+1$ & $2$ & $2$ & $p+q-2$ & $q-1$ & $0$\\
  II$.5$ & $\Herm(3,\OO_s)$ & $3$ & $27$ & $15$ & $3$ & $3$ & $8$ & $4$ & $0$\\
  \hline
  III$.1$ & $\Sym(n,\CC)$ & $1$ & $n(n+1)$ & $\frac{n}{2}(n+1)$ & $2n$ & $n$ & $2$ & $1$ & $1$\\
  III$.2$ & $M(n,\CC)$ & $2$ & $2n^2$ & $n^2$ & $2n$ & $n$ & $4$ & $2$ & $1$\\
  III$.3$ & $\Skew(2n,\CC)$ & $3$ & $2n(2n-1)$ & $n(2n-1)$ & $2n$ & $n$ & $8$ & $4$ & $1$\\
  III$.4$ & $\CC^n$ ($n\geq3$) & $4$ & $2n$ & $n$ & $4$ & $2$ & $2(n-2)$ & $n-2$ & $1$\\
  III$.5$ & $\Herm(3,\OO)^\CC$ & $5$ & $54$ & $27$ & $6$ & $3$ & $16$ & $8$ & $1$\\
  \hline
  IV$.1$ & $\Sym(2n,\CC)\cap M(n,\HH)$ & $2$ & $n(2n+1)$ & $n^2$ & $2n$ & $n$ & $4$ & $2$ & $2$\\
  IV$.2$ & $M(n,\HH)$ & $3$ & $4n^2$ & $n(2n-1)$ & $2n$ & $n$ & $8$ & $4$ & $3$\\
  IV$.3$ & $\times\times\times$ & $\times$ & $\times$ & $\times$ & $\times$ & $\times$ & $\times$ & $\times$ & $\times$\\
  IV$.4$ & $\RR^{n,0}$ ($n\geq2)$ & $4$ & $n$ & $1$ & $2$ & $1$ & $0$ & $0$ & $n-1$\\
  IV$.5$ & $\times\times\times$ & $\times$ & $\times$ & $\times$ & $\times$ & $\times$ & $\times$ & $\times$ & $\times$\\
  \hline
\end{tabular}
\caption{Structure constants}
\label{tb:Constants}
\end{center}
\end{table}

\section{The constants $\mu$ and $\nu$}

\begin{table}
\begin{center}
\begin{tabular}[ht]{|r|c|c|c|}
  \hline
  & $V$ & $\mu$ & $\nu$\\
  \hline
  I$.1$ & $\Sym(n,\RR)$ & $(n-2)/2$ & $-1$\\
  I$.2$ & $\Herm(n,\CC)$ & $n-1$ & $-1$\\
  I$.3$ & $\Herm(n,\HH)$ & $2n-1$ & $-1$\\
  I$.4$ & $\RR^{1,n-1}$ ($n\geq3$) & $n-3$ & $-1$\\
  I$.5$ & $\Herm(3,\OO)$ & $11$ & $-1$\\
  \hline
  II$.1$ & $\times\times\times$ & $\times$ & $\times$\\
  II$.2$ & $M(n,\RR)$ & $n-2$ & $0$\\
  II$.3$ & $\Skew(2n,\RR)$ & $2n-3$ & $1$\\
  II$.4$ & $\RR^{p,q}$ ($p,q\geq2$) & $\max(p,q)-2$ & $\min(p,q)-2$\\
  II$.5$ & $\Herm(3,\OO_s)$ & $7$ & $3$\\
  \hline
  III$.1$ & $\Sym(n,\CC)$ & $n-1$ & $-1$\\
  III$.2$ & $M(n,\CC)$ & $2(n-1)$ & $0$\\
  III$.3$ & $\Skew(2n,\CC)$ & $2(2n-2)$ & $2$\\
  III$.4$ & $\CC^n$ ($n\geq3$) & $n-2$ & $n-4$\\
  III$.5$ & $\Herm(3,\OO)^\CC$ & $16$ & $6$\\
  \hline
  IV$.1$ & $\Sym(2n,\CC)\cap M(n,\HH)$ & $2n-1$ & $-1$\\
  IV$.2$ & $M(n,\HH)$ & $4n-2$ & $0$\\
  IV$.3$ & $\times\times\times$ & $\times$ & $\times$\\
  IV$.4$ & $\RR^{n,0}$ ($n\geq2$) & $n-2$ & $-n$\\
  IV$.5$ & $\times\times\times$ & $\times$ & $\times$\\
  \hline
\end{tabular}
\caption{The constants $\mu$ and $\nu$}
\label{tb:Parameters}
\end{center}
\end{table}

\section{Conformal algebra and structure algebra}

\begin{table}
\begin{center}
\begin{tabular}[ht]{|r|c|c|c|}
  \hline
  & $V$ & $\frakg=\co(V)$ & $\frakl=\str(V)$\\
  \hline
  I$.1$ & $\Sym(n,\RR)$ & $\sp(n,\RR)$ & $\sl(n,\RR)\times\RR$\\
  I$.2$ & $\Herm(n,\CC)$ & $\su(n,n)$ & $\sl(n,\CC)\times\RR$\\
  I$.3$ & $\Herm(n,\HH)$ & $\so^*(4n)$ & $\sl(n,\HH)\times\RR$\\
  I$.4$ & $\RR^{1,n-1}$ ($n\geq3$) & $\so(2,n)$ & $\so(1,n-1)\times\RR$\\
  I$.5$ & $\Herm(3,\OO)$ & $\mathfrak{e}_{7(-25)}$ & $\mathfrak{e}_{6(-26)}\times\RR$\\
  \hline
  II$.1$ & $\times\times\times$ & $\times\times\times$ & $\times\times\times$\\
  II$.2$ & $M(n,\RR)$ & $\sl(2n,\RR)$ & $\sl(n,\RR)\times\sl(n,\RR)\times\RR$\\
  II$.3$ & $\Skew(2n,\RR)$ & $\so(2n,2n)$ & $\sl(2n,\RR)\times\RR$\\
  II$.4$ & $\RR^{p,q}$ ($p,q\geq2$) & $\so(p+1,q+1)$ & $\so(p,q)\times\RR$\\
  II$.5$ & $\Herm(3,\OO_s)$ & $\mathfrak{e}_{7(7)}$ & $\mathfrak{e}_{6(6)}\times\RR$\\
  \hline
  III$.1$ & $\Sym(n,\CC)$ & $\sp(n,\CC)$ & $\sl(n,\CC)\times\CC$\\
  III$.2$ & $M(n,\CC)$ & $\sl(2n,\CC)$ & $\sl(n,\CC)\times\sl(n,\CC)\times\CC$\\
  III$.3$ & $\Skew(2n,\CC)$ & $\so(4n,\CC)$ & $\sl(2n,\CC)\times\CC$\\
  III$.4$ & $\CC^n$ ($n\geq3$) & $\so(n+2,\CC)$ & $\so(n,\CC)\times\CC$\\
  III$.5$ & $\Herm(3,\OO)^\CC$ & $\mathfrak{e}_7(\CC)$ & $\mathfrak{e}_6(\CC)\times\CC$\\
  \hline
  IV$.1$ & $\Sym(2n,\CC)\cap M(n,\HH)$ & $\sp(n,n)$ & $\sl(n,\HH)\times\HH$\\
  IV$.2$ & $M(n,\HH)$ & $\sl(2n,\HH)$ & $\sl(n,\HH)\times\sl(n,\HH)\times\HH$\\
  IV$.3$ & $\times\times\times$ & $\times\times\times$ & $\times\times\times$\\
  IV$.4$ & $\RR^{n,0}$ ($n\geq2$) & $\so(1,n+1)$ & $\so(n)\times\RR$\\
  IV$.5$ & $\times\times\times$ & $\times\times\times$ & $\times\times\times$\\
  \hline
\end{tabular}
\caption{Conformal algebra and structure algebra}
\label{tb:Groups}
\end{center}
\end{table}

\chapter{Some calculations}

\begin{lemma}\label{lem:BracketZero}
\begin{enumerate}
\item[\textup{(1)}] Let $c\in V$ be an idempotent. Then for any $u\in V(c,1)$:
\begin{align*}
 [L(c),L(u)] &= 0.
\end{align*}
\item[\textup{(2)}] Let $c_1,c_2\in V$ be orthogonal idempotents. Then for any $u\in V(c_1,\frac{1}{2})\cap V(c_2,\frac{1}{2})$:
\begin{align*}
 [L(c_1),L(u)] &= -[L(c_2),L(u)].
\end{align*}
\end{enumerate}
\end{lemma}

\begin{proof}
(2) follows directly from (1) with $c:=c_1+c_2$. For (1) we find, using \cite[Proposition II.1.1 (i)]{FK94}:
\begin{align*}
 [L(u),L(c)] &= [L(u),L(c^2)] = -2[L(c),L(uc)]\\
 &= -2[L(c),L(u)] = 2[L(u),L(c)]
\end{align*}
which gives the claim.
\end{proof}

\begin{lemma}\label{lem:SquareSums}
Let $(e_\alpha)_\alpha$ be an orthonormal basis of $V$ with respect to $(-|-)$ and $(\overline{e}_\alpha)_\alpha$ the dual basis with respect to the trace form $\tau(-,-)$, i.e. $\overline{e}_\alpha=\alpha(e_\alpha)$. Then
\begin{align*}
 \sum_\alpha{e_\alpha^2} &= \frac{2n_0-n}{r}e &\mbox{and} && \sum_\alpha{e_\alpha\cdot\overline{e}_\alpha} &= \frac{n}{r}e.
\end{align*}
\end{lemma}

\begin{proof}
It is easily seen that the elements $\sum_\alpha{e_\alpha^2}$ and $\sum_\alpha{e_\alpha\cdot\overline{e}_\alpha}$ are independent of the orthonormal basis. Since the Peirce decomposition $V=\oplus_{i\leq j}{V_{ij}}$ is orthogonal with respect to $(-|-)$, we can choose an orthonormal basis $(e_\alpha)_\alpha$ such that each $e_\alpha$ is contained in one of the $V_{ij}$, $i\leq j$. Furthermore, since $\alpha$ leaves each $V_{ij}$, $i\leq j$, invariant, we can even choose the $e_\alpha$ to be either in $(V_{ij})_0:=V_{ij}\cap V_0$ or in $(V_{ij})_1:=V_{ij}\cap V_1$.
\begin{enumerate}
 \item[\textup{(a)}] Let $e_\alpha\in (V_{ii})_0$. Then $e_\alpha=\lambda c_i$ with $\lambda=\|c_i\|^{-1}=\left(\frac{r_0}{r}\right)^{\frac{1}{2}}$. Hence
 \begin{align*}
  e_\alpha^2 &= \frac{r_0}{r}c_i & \mbox{and } & & \dim(V_{ii})_0 &= 1.
 \end{align*}
 \item[\textup{(b)}] Let $e_\alpha\in (V_{ii})_1$. Then $e_\alpha^2\in (V_{ii})_0=\RR c_i$ and therefore $e_\alpha^2=\lambda c_i$. Since
 \begin{align*}
  1 &= \|e_\alpha\|^2 = (e_\alpha|e_\alpha) = -\tau(e_\alpha|e_\alpha)\\
  &= -\tau(e_\alpha^2|e) = -\lambda\tau(c_i|e) = -\lambda\|c_i\|^2 = -\lambda\frac{r}{r_0},
 \end{align*}
 we obtain
 \begin{align*}
  e_\alpha^2 &= -\frac{r_0}{r}c_i & \mbox{and } & & \dim(V_{ii})_1 &= e.
 \end{align*}
 \item[\textup{(c)}] Let $e_\alpha\in (V_{ij})_0$, $i<j$. Then $e_\alpha^2\in (V_{ii})_0+(V_{jj})_0$ and hence $e_\alpha^2=\lambda c_i+\mu c_j$. Similar to the calculation in (b) one obtains
 \begin{align*}
  e_\alpha^2 &= \frac{r_0}{2r}(c_i+c_j) & \mbox{and } & & \dim(V_{ij})_0 &= d_0.
 \end{align*}
 \item[\textup{(d)}] Let $e_\alpha\in (V_{ij})_1$, $i<j$. Applying the same arguments as in (b) and (c) yields
 \begin{align*}
  e_\alpha^2 &= -\frac{r_0}{2r}(c_i+c_j) & \mbox{and } & & \dim(V_{ij})_0 &= d-d_0.
 \end{align*}
\end{enumerate}
Putting everything together gives
\begin{align*}
 \sum_\alpha{e_\alpha^2} &= \sum_{i=1}^{r_0}{\sum_{e_\alpha\in V_{ii}}{e_\alpha^2}} + \sum_{1\leq i<j\leq r_0}{\sum_{e_\alpha\in V_{ij}}{e_\alpha^2}}\\
 &= \frac{r_0}{r}\sum_{i=1}^{r_0}{(1-e)c_i} + \frac{r_0}{r}\sum_{1\leq i<j\leq r_0}{\frac{1}{2}(d_0-(d-d_0))(c_i+c_j)}\\
 &= \frac{r_0}{r}\left(2\left(1+(r_0-1)\frac{d_0}{2}\right)-\left(e+1+(r_0-1)\frac{d}{2}\right)\right)\sum_{i=1}^{r_0}{c_i}\\
 &= \frac{2n_0-n}{r}e.
\end{align*}
A similar calculation also gives the second formula.
\end{proof}

\begin{corollary}\label{cor:QRepC}
Let $c\in V_0$ be a primitive idempotent and $(e_\alpha)_\alpha$ an orthonormal basis of $V$ with respect to $(-|-)$. Then
\begin{align*}
 \sum_\alpha{P(e_\alpha)c} &= \frac{r_0}{r}\left(\frac{d}{2}-d_0-e+1\right)c + \frac{r_0}{r}\left(d_0-\frac{d}{2}\right)e.
\end{align*}
\end{corollary}

\begin{proof}
Again it is easily seen that the expression $\sum_\alpha{P(e_\alpha)c}$ is independent of the chosen orthonormal basis. Since the Peirce decomposition $V=V(c,1)\oplus V(c,\frac{1}{2})\oplus V(c,0)$ is orthogonal with respect to $(-|-)$, we can choose the orthonormal basis $(\overline{e}_\alpha)_\alpha$ such that $\overline{e}_\alpha\in V(c,1)\cup V(c,\frac{1}{2})\cup V(c,0)$ for every $\alpha$. Then, by Proposition ???, the $e_\alpha\in V(c,1)$ form an orthonormal basis of $V(c,1)$ and those $e_\alpha\in V(c,0)=V(e-c,1)$ form an orthonormal basis of $V(c,0)$. Now let us determine the action of $P(e_\alpha)$ on $c$ for the following three cases.
\begin{enumerate}
 \item[\textup{(a)}] $e_\alpha\in V(c,1)$. Since $V(c,1)$ is a subalgebra, also $e_\alpha^2\in V(c,1)$. Hence
 \begin{align*}
  P(e_\alpha)c &= 2e_\alpha(e_\alpha c)-e_\alpha^2c = 2e_\alpha^2-e_\alpha^2=e_\alpha^2.
 \end{align*}
 \item[\textup{(b)}] $e_\alpha\in V(c,\frac{1}{2})$. In this case
 \begin{align*}
  P(e_\alpha)c &= 2e_\alpha(e_\alpha c)-e_\alpha^2c = e_\alpha^2 - e_\alpha^2c = (e-c)e_\alpha^2.
 \end{align*}
 \item[\textup{(c)}] $e_\alpha\in V(c,0)$. Also $V(c,0)=V(e-c,1)$ is a subalgebra and hence $e_\alpha^2\in V(c,0)$. Then clearly
 \begin{align*}
  P(e_\alpha)c &= 2e_\alpha(e_\alpha c)-e_\alpha^2c = 0.
 \end{align*}
\end{enumerate}
Altogether we obtain
\begin{align*}
 \sum_\alpha{P(\overline{e}_\alpha)c} &= \sum_{\begin{subarray}{c}\alpha\\\overline{e}_\alpha\in V(c,1)\end{subarray}}{\overline{e}_\alpha^2} + (e-c)\sum_{\begin{subarray}{c}\alpha\\\overline{e}_\alpha\in V(c,\frac{1}{2})\end{subarray}}{\overline{e}_\alpha^2}\\
 &= (e-c)\sum_\alpha{\overline{e}_\alpha^2} + \sum_{\begin{subarray}{c}\alpha\\\overline{e}_\alpha\in V(c,1)\end{subarray}}{\overline{e}_\alpha^2} - \sum_{\begin{subarray}{c}\alpha\\\overline{e}_\alpha\in V(c,0)\end{subarray}}{\overline{e}_\alpha^2}.
\end{align*}
Put $n_c:=\dim\,V(c,1)$, $n_{c,0}:=\dim(V(c,1)\cap V_0)$, $r_c:=\rank\,V(c,1)$ and similar for $e-c$. Then, using Lemma \ref{lem:SquareSums}:
\begin{align*}
 \sum_\alpha{P(\overline{e}_\alpha)c} &= \frac{2n_0-n}{r}(e-c) + \frac{2n_{c,0}-n_c}{r_c}c - \frac{2n_{e-c,0}-n_{e-c}}{r_{e-c}}(e-c)\\
 &= \frac{r_0}{r}\left(\frac{d}{2}-d_0-e+1\right)c + \frac{r_0}{r}\left(d_0-\frac{d}{2}\right)e.\qedhere
\end{align*}
\end{proof}

\begin{lemma}
Let $(e_j)_j\subseteq V$ be an orthonormal basis of $V$ with respect to the inner product $(-|-)$. Then for $x\in V$:
\begin{align}
 \sum_{j=1}^n{\tau(P(\alpha x,\alpha e_j)x,e_j)} &= \frac{n}{r}\|x\|^2.\label{eq:SumQuadRep}
\end{align}
\end{lemma}

\begin{proof}
\begin{align*}
 \sum_{j=1}^n{\tau(P(\alpha x,\alpha e_j)x,e_j)} &= \sum_{j=1}^n{\tau((\alpha x\square x)(\alpha e_j),e_j)}\\
 &= \sum_{j=1}^n{((x\square\alpha x)e_j|e_j)} = \Tr(x\square\alpha x)\\
 &= \Tr(L(x\cdot\alpha x)+[L(x),L(\alpha x)]) = \Tr(L(x\cdot\alpha x))\\
 &= \frac{n}{r}\tr(x\cdot\alpha x) = \frac{n}{r}(x|x) = \frac{n}{r}\|x\|^2
\end{align*}
by Lemma \ref{lem:Trtr}.
\end{proof}

\begin{proposition}
The rank of $V(c_j,1)$ is $j\frac{r}{r_0}$.
\end{proposition}

\begin{proof}
This is clear by \cite[Section 8, Korollar 2]{Hel69}.
\end{proof}

\begin{corollary}
Let $c$ be an idempotent in $V$. Then
\begin{align*}
 \tr_V(x) &= \tr_{V(c,1)}(x)+\tr_{V(c,0)}(x), & \forall x\in V.
\end{align*}
\end{corollary}

\begin{proof}
The trace is $=0$ on $e^\perp$ and on the euclidean part $V_0$ which contains $e$, $c$ and $e-c$ one can use the uniqueness result of \cite[Proposition III.4.1]{FK94}.
\end{proof}

\begin{corollary}\label{cor:IdempotentNorm}
Let $c$ be a primitive idempotent, then $\|c\|^2=\frac{r}{r_0}$.
\end{corollary}

\chapter{Calculations in rank $2$}\label{sec:Rank2Kfinite}

Let $V=\RR^{p,q}$ with $p,q\geq1$ (see Example \ref{ex:JordanAlgebras} (2)). The structure constants of $V$ can be found in Table \ref{tb:Constants} where $V$ corresponds to the case II.4. In particular, $V$ has dimension $n=p+q$ and rank $r=r_0=2$. The parameter of the Riesz distribution corresponding to the minimal orbit of $L$ is $\lambda_1=\frac{r_0d}{2r}=\frac{p+q-2}{2}$. Let us for convenience assume that $p\leq q$. (The case $p\geq q$ can be treated similarly.) Then $\mu=q-2$ and $\nu=p-2$.

Denote by $(e_i)_{i=1,\ldots,n}$ the standard basis of $V=\RR^n$. We will use coordinates $x_1,\ldots,x_n$ for $x=\sum_{i=1}^n{x_ie_i}$. In these coordinates the trace form and the determinant are given by
\begin{align*}
 \tau(x,y) &= 2(x_1y_1-x_2y_2-\ldots-x_py_p+x_{p+1}y_{p+1}+\ldots+x_ny_n),\\
 \Delta(x) &= x_1^2+\ldots+x_p^2-x_{p+1}^2-\ldots-x_n^2.
\end{align*}
Hence, $\alpha e_i:=\epsilon_ie_i$ defines a Cartan involution of $V$, where
\begin{align*}
 \epsilon_i := \begin{cases}+1 & \mbox{for $i=1$ or $i=p+1,\ldots,n$,}\\-1 & \mbox{for $i=2,\ldots,p$.}\end{cases}
\end{align*}
The basis dual to $(e_i)$ with respect to the trace form $\tau$ is therefore given by $\overline{e}_i=\frac{1}{2}\epsilon_ie_i$. The corresponding inner product and norm are
\begin{align*}
 (x|y) &= \tau(x,\alpha y) = 2(x_1y_1+\ldots+x_ny_n),\\
 |x|^2 &= \|x\|^2 = 2(x_1^2+\ldots+x_n^2).
\end{align*}
The gradient $\frac{\partial}{\partial x}$ with respect to the trace form writes
\begin{align*}
 \frac{\partial}{\partial x} &= \left(\frac{\epsilon_j}{2}\frac{\partial}{\partial x_j}\right)_j = \frac{1}{2}\left(\frac{\partial}{\partial x_1},-\frac{\partial}{\partial x_2},\ldots,-\frac{\partial}{\partial x_p},\frac{\partial}{\partial x_{p+1}},\ldots,\frac{\partial}{\partial x_n}\right).
\end{align*}
Further, an orthonormal basis of $V$ with respect to the inner product $(-|-)$ is given by the vectors $\frac{1}{\sqrt{2}}e_i$ ($i=1,\ldots,n$). We also fix the Jordan frame $c_1:=\frac{1}{2}(e_1+e_{p+q})$, $c_2:=\frac{1}{2}(e_1-e_{p+q})$.

Let us use the notation $x=(x',x'')\in\RR^ p\times\RR^ q$ for $x\in V$. By $x'$ and $x''$ we will also denote the vectors $(x',0)\in V$ and $(0,x'')\in V$, respectively. In this notation the minimal orbit $\calO_1$ can be written as
\begin{align*}
 \calO_1 &= \{x\in V\setminus\{0\}: \Delta(x)=0\}\\
 &= \{(x',x'')\in V\setminus\{0\}: |x'|=|x''|\}.
\end{align*}
In particular, for $x=(x',x'')\in\calO_1$ we have $|x'|^2=|x''|^2=\frac{1}{2}|x|^2$.

Now let us calculate the action of the Bessel operator $\calB_\lambda$ ($\lambda=\lambda_1$) in this case. To apply Proposition \ref{prop:BnuRadial} we have to calculate $ke$ for $k\in M=\SO(p)\times\SO(q)$. One finds that for $x=ktc_1\in\calO_1$ with $t>0$, $k\in M$ we have $kte=(2x',0)$. Hence we obtain for $\psi(x)=f(|x|)$:
\begin{align*}
 \calB_\lambda\psi(x) &= \left(f''(|x|)+d_0\frac{1}{|x|}f'(|x|)\right)\alpha(x')+\left(f''(|x|)+(d-d_0)\frac{1}{|x|}f'(|x|)\right)\alpha(x'').
\end{align*}
For the action of the Lie algebra elements $(e_i,0,-\alpha e_i)\in\frakk$ this yields
\begin{multline}
 \td\pi_\lambda(e_j,0,-\alpha e_j)\psi(x)\\
 = \begin{cases}\frac{1}{i}\left(f''(|x|)+(q-1)\frac{1}{|x|}f'(|x|)-f(|x|)\right)(x|e_j) & \mbox{for $1\leq j\leq p$,}\\\frac{1}{i}\left(f''(|x|)+(p-1)\frac{1}{|x|}f'(|x|)-f(|x|)\right)(x|e_j) & \mbox{for $p+1\leq j\leq n$.}\end{cases}\label{eq:kActionRank2}
\end{multline}

\section{The minimal $K$-type}

In this section we prove the remaining parts (b) and (c) of Proposition \ref{prop:Kfinite}. For this we introduce operators for $j=1,\ldots,p$:
\begin{align*}
 (-)^+_j:\calH^k(\RR^p) &\rightarrow \calH^{k+1}(\RR^p), & \varphi^+_j(x) &:= x_j\varphi(x)-\frac{x_1^2+\ldots+x_p^2}{p+2k-2}\frac{\partial\varphi}{\partial x_j},\\
 (-)^-_j:\calH^k(\RR^p) &\rightarrow \calH^{k-1}(\RR^p), & \varphi^-_j(x) &:= \frac{1}{p+2k-2}\frac{\partial\varphi}{\partial x_j}.
\end{align*}
That $\varphi^+_j$ and $\varphi^-_j$ are indeed homogeneous harmonic polynomials of degree $k+1$ and $k-1$, respectively, can easily be checked by direct computation. Then one clearly has the following decomposition of $x_j\varphi(x)$ into spherical harmonics:
\begin{align*}
 x_j\varphi(x) &= \varphi^+_j(x)+(x_1^2+\ldots+x_p^2)\varphi_j^-(x).
\end{align*}
For convenience we also put $(-)^+_j:=(-)^-_j:=0$ for $j=p+1,\ldots,n$. Using the operators $(-)^+_j$ and $(-)^-_j$ we prove the following lemma:

\begin{lemma}\label{lem:Rank2KAction}
For $j=1,\ldots,n$ the action of $(e_j,0,-\alpha e_j)\in\frakk$ on $\widetilde{K}_{\frac{\nu}{2}+k}\otimes\varphi\in\widetilde{K}_{\frac{\nu}{2}+k}\otimes\calH^k(\RR^p)$ is given by
\begin{multline*}
 \td\pi_\lambda(e_j,0,-\alpha e_j)(\widetilde{K}_{\frac{\nu}{2}+k}\otimes\varphi)\\
 = \frac{1}{i}\left[(2k+p-q)\widetilde{K}_{\frac{\nu}{2}+k+1}\otimes\varphi_j^+-(2k+p+q-4)\widetilde{K}_{\frac{\nu}{2}+k-1}\otimes\varphi_j^-\right].
\end{multline*}
\end{lemma}

\begin{proof}
Let $\varphi\in\calH^k(\RR^p)$ and $1\leq j\leq n$. With the product rule \eqref{eq:drhoProdRule} and \eqref{eq:ddxradial} we obtain
\begin{multline*}
 \td\pi_\lambda(e_j,0,-\alpha e_j)(\widetilde{K}_{\frac{\nu}{2}+k}\otimes\varphi)(x) = \td\pi_\lambda(e_j,0,-\alpha e_j)\widetilde{K}_{\frac{\nu}{2}+k}(x)\cdot\varphi(x)\\
 +\frac{2}{i}\frac{\widetilde{K}_{\frac{\nu}{2}+k}'(|x|)}{|x|}\tau\left(P\left(\alpha x,\frac{\partial\varphi}{\partial x}\right)x,e_j\right)+\frac{1}{i}\widetilde{K}_{\frac{\nu}{2}+k}(|x|)\tau(\calB_\lambda\varphi(x),e_j).
\end{multline*}
Using the two identities
\begin{align*}
 \sum_{j=1}^p{x_j\frac{\partial\varphi}{\partial x_j}(x)} &= k\varphi(x) & \mbox{and} && \sum_{j=1}^p{\frac{\partial^2\varphi}{\partial x_j^2}}=0
\end{align*}
a short calculation gives
\begin{align*}
 P\left(\alpha x,\frac{\partial\varphi}{\partial x}\right)x &= k\varphi(x')x''+\frac{1}{2}|x|^2\frac{\partial\varphi}{\partial x}(x'),\\
 \calB_\lambda\varphi &= (\lambda+k-1)\frac{\partial\varphi}{\partial x}.
\end{align*}
\begin{enumerate}
\item[\textup{(a)}] $j=1,\ldots,p$. With \eqref{eq:kActionRank2} and the differential equation \eqref{eq:DiffEqModBessel} we obtain
\begin{multline*}
 \td\pi_\lambda(e_j,0,-\alpha e_j)(\widetilde{K}_{\frac{\nu}{2}+k}\otimes\varphi)(x) = \frac{1}{i}\left[-2(2k+p-q)\frac{1}{|x|}\widetilde{K}_{\frac{\nu}{2}+k}'(|x|)\cdot x_j\varphi(x)\right.\\
 \left.+ |x|\widetilde{K}_{\frac{\nu}{2}+k}'(|x|)\cdot\frac{\partial\varphi}{\partial x_j}(x) + \left(k+\frac{p+q-4}{2}\right)\widetilde{K}_{\frac{\nu}{2}+k}(|x|)\cdot\frac{\partial\varphi}{\partial x_j}(x)\right].
\end{multline*}
Applying \eqref{eq:KBesselDiffRecRel} and \eqref{eq:KBesselRecRel} yields the stated formula.
\item[\textup{(b)}] $j=p+1,\ldots,n$. In this case $\tau(\frac{\partial\varphi}{\partial x},e_j)=0$ and $\tau(x'',e_j)=(x|e_j)$. Using again \eqref{eq:kActionRank2} we find that
\begin{multline*}
 \td\pi_\lambda(e_j,0,-\alpha e_j)(\widetilde{K}_{\frac{\nu}{2}+k}\otimes\varphi)(x)\\
 = \frac{1}{i}\left[\widetilde{K}_{\frac{\nu}{2}+k}''(|x|)+(2k+p-1)\frac{1}{|x|}\widetilde{K}_{\frac{\nu}{2}+k}'(|x|)-\widetilde{K}_{\frac{\nu}{2}+k}(|x|)\right](x|e_j)\varphi(x).
\end{multline*}
But this is $=0$ by \eqref{eq:DiffEqModBessel} which finishes the proof.\qedhere
\end{enumerate}
\end{proof}

Now
\begin{align*}
 \frakk = \frakm \oplus \{(u,0,-\alpha u):u\in V\}
\end{align*}
and $\frakm=\frako(p)\oplus\frako(q)$ acts irreducibly on $\calH^k(\RR^p)$ for every $k\geq0$. Therefore, the previous Lemma implies that
\begin{align*}
 W_0 &= \begin{cases}\displaystyle\bigoplus_{k=0}^{\frac{q-p}{2}}{\widetilde{K}_{\frac{\nu}{2}+k}\otimes\calH^k(\RR^p)} & \mbox{if $q-p\in2\ZZ$,}\\\displaystyle\bigoplus_{k=0}^\infty{\widetilde{K}_{\frac{\nu}{2}+k}\otimes\calH^k(\RR^p)} & \mbox{else,}\end{cases}
\end{align*}
which finishes the proof of Proposition \ref{prop:Kfinite}.\\

Next we want to determine the highest weight of $W_0$. For this we first give an explicit isomorphism between $\frakk$ and $\frako(p+1)\oplus\frako(q+1)$. Here we realize $\frako(p+1)\oplus\frako(q+1)$ in the space of $(n+2)\times(n+2)$ matrices by
\begin{align*}
 \frako(p+1)\oplus\frako(q+1) = \left(\begin{array}{cc}\frako(p+1) & 0\\0 & \frako(q+1)\end{array}\right)
\end{align*}
Then it is easy to check that
\begin{align*}
 (0,T,0) &\mapsto \left(\begin{array}{c|c|c}0&&\\\hline&T&\\\hline&&0\end{array}\right), && T\in\frakm=\frako(p)\oplus\frako(q),\\
 (x,0,-\alpha x) &\mapsto \left(\begin{array}{c|c|c|c}0&2x'^t&&\\\hline-2x'&0&&\\\hline&&0&-2x''\\\hline&&2x''^t&0\end{array}\right), && x\in V,
\end{align*}
defines an isomorphism $\frakk\stackrel{\sim}{\rightarrow}\frako(p+1)\oplus\frako(q+1)$ of Lie algebras.

\begin{lemma}\label{lem:IdentLowestKtypeRk2}
Under the identification $\frakk\cong\frako(p+1)\oplus\frako(q+1)$ the map
\begin{align*}
 \varphi:\sum_{k=0}^{\frac{q-p}{2}}{\widetilde{K}_{\frac{\nu}{2}+k}\otimes\calH^k(\RR^p)}&\rightarrow\calH^{\frac{q-p}{2}}(\RR^{p+1}),\\
 \varphi\left(\widetilde{K}_{\frac{\nu}{2}+k}\otimes\varphi\right)(x_0,x')&:=\frac{(-2i)^k}{(\frac{p-q}{2})_k}\widetilde{C}_{\frac{q-p}{2}-k}^{\frac{p-1}{2}+k}(x_0)\varphi(x'), & (x_0,x')\in\SS^p\subseteq\RR^{p+1}.
\end{align*}
becomes an isomorphism of $\frakk$-modules.
\end{lemma}

Here $\widetilde{C}_n^\lambda(z)=\Gamma(\lambda)C_n^\lambda(z)$ denotes the normalized Gegenbauer polynomials and $(a)_k=a(a+1)\cdots(a+k-1)$ the Pochhammer symbol.

\begin{proof}
The action of $A\in\frako(p+1)$ on $\psi\in\calH^{\frac{q-p}{2}}(\RR^{p+1})$ is given by
\begin{align*}
 (A\cdot\psi)(x) &:= D_{A^*x}\psi(x) = -D_{Ax}\psi(x).
\end{align*}
Then it is clear that $\varphi$ intertwines the actions of $\frako(p)\subseteq\frakm$. It remains to check that it also intertwines the actions of $(e_j,0,-\alpha e_j)$ for $1\leq j\leq p$. To prove this, we make use of the following two formulas for the normalized Gegenbauer polynomials (cf \cite[equations (6.4.15) and (6.4.16)]{AAR99}):
\begin{align}
 \frac{\td}{\td z}\widetilde{C}_n^\lambda(z) = 2\widetilde{C}_{n-1}^{\lambda+1}(z)\label{eq:Gegenbauer1}\\
 (2\lambda+n-1)(n+1)\widetilde{C}_{n+1}^{\lambda-1}(z)&-2z(2\lambda-1)\widetilde{C}_n^\lambda(z)+4(1-z^2)\widetilde{C}_{n-1}^{\lambda+1}(z) = 0.\label{eq:Gegenbauer2}
\end{align}
We then have for $(x_0,x')\in\SS^p$:
\begin{align*}
 & \left((e_j,0,-\alpha e_j)\cdot\varphi(\widetilde{K}_{\frac{\nu}{2}+k}\otimes\varphi)\right)(x_0,x')\\
 ={}& \left(-2x_j\frac{\partial}{\partial x_0}+2x_0\frac{\partial}{\partial x_j}\right)\varphi(\widetilde{K}_{\frac{\nu}{2}+k}\otimes\varphi)(x_0,x')\\
 \stackrel{\eqref{eq:Gegenbauer1}}{=}{}& -4\frac{(-2i)^k}{(\frac{p-q}{2})_k}\widetilde{C}_{\frac{q-p}{2}-(k+1)}^{\frac{p-1}{2}+(k+1)}(x_0)x_j\varphi(x')+2\frac{(-2i)^k}{(\frac{p-q}{2})_k}x_0\widetilde{C}_{\frac{q-p}{2}-k}^{\frac{p-1}{2}+k}(x_0)\frac{\partial\varphi}{\partial x_j}(x')\\
 \stackrel{\eqref{eq:Gegenbauer2}}{=}{}& \frac{1}{i}\left[(2k+p-q)\varphi(\widetilde{K}_{\frac{\nu}{2}+(k+1)}\otimes\varphi_j^+)-(2k+p+q-4)\varphi(\widetilde{K}_{\frac{\nu}{2}+(k-1)}\otimes\varphi_j^-)\right](x_0,x')\\
 ={}& \varphi\left((e_j,0,-\alpha e_j)\cdot(\widetilde{K}_{\frac{\nu}{2}+k}\otimes\varphi)\right)(x_0,x')
\end{align*}
by Lemma \ref{lem:Rank2KAction}.
\end{proof}

We use the identification $\frakk\cong\frako(p+1)\oplus\frako(q+1)$ to transfer the maximal torus, roots and our choice of a positive system for $\frakk$ to $\frako(p+1)\oplus\frako(q+1)$. Then by \cite[IV.7, Examples (1) \& (2)]{Kna86} the function $\psi(x)=(x_0+ix_1)^{\frac{q-p}{2}}$ is a highest weight vector in $\calH^{\frac{q-p}{2}}(\RR^{p+1})$ and the corresponding highest weight is given by
\begin{align*}
 \epsilon\left(\begin{array}{cc|ccc}0&a&&&\\-a&0&&&\\\hline&&*&&\\&&&\ddots&\\&&&&*\end{array}\right) &= \frac{q-p}{2}ia.
\end{align*}
Under the above identification $\epsilon$ corresponds to $\frac{q-p}{4}(\gamma_1+\gamma_2)$ which is in turn the highest weight of the $\frakk$-module $W_0$. This proves Proposition \ref{prop:HighestWeightW0}.\\

Finally we calculate the action of $\calF_\calO=\pi(w_0)$ on the minimal $K$-type $W_0$. Since $w_0=j\alpha$ is in the center of $K$, $\pi(w_0)$ acts on $W_0$ as a scalar. We determine this scalar by applying $\pi(w_0)$ to $\psi_0$. First, $\pi(\alpha)\psi_0=\psi_0$ as $\alpha\in M$ and $\psi$ is $M$-invariant. Therefore, we have to calculate $\pi(j)\psi_0$. Under the identification $K_0\cong SO(p+1)\times SO(q+1)$ the element $j\in K_0$ corresponds to the matrix
\begin{align*}
 \left(\begin{array}{cc}-\1_2&0\\0&\1_{p+q-2}\end{array}\right).
\end{align*}
And by Lemma \ref{lem:IdentLowestKtypeRk2} the function $\psi_0\in W_0$ corresponds to the function
\begin{align*}
 \SS^p\mapsto\CC, (x_0,x')\mapsto\widetilde{C}_{\frac{q-p}{2}}^{\frac{p-1}{2}}(x_0).
\end{align*}
In view of the following parity formula for the Gegenbauer polynomials (follows e.g. from \cite[equation (6.4.12)]{AAR99}):
\begin{align*}
 \widetilde{C}_n^\lambda(-z) &= (-1)^n\widetilde{C}_n^\lambda(z),
\end{align*}
we see that $\pi(j)\psi_0=(-1)^{\frac{q-p}{2}}\psi_0$. This finishes the proof of Proposition \ref{prop:AkkappaPsi0}.

\section{The Casimir action}

In this section we calculate the Casimir action in the rank $2$ case. The action of $(e_j,0,-\alpha e_j)$ on radial functions is given in \eqref{eq:kActionRank2}. Note that $(e_j)_j$ denotes the standard basis of $\RR^n$ which is not orthonormal with respect to the inner product $(-|-)$. With the notation of \eqref{eq:1dimBesselOp} we find that for $x\in\calO_1$:
\begin{align*}
& -\sum_{j=1}^p{\td\pi(e_j,0,-\alpha e_j)^2\psi(x)}\\
 \stackrel{\eqref{eq:BnuProdRule}}{=}{}& \sum_{j=1}^p{\left[(B_{q-2}^2f)(|x|)(x|e_j)^2+2\tau\left(\left.P\left(\frac{\partial(B_{q-2}f)}{\partial x}\right|\frac{\partial(x|e_j)}{\partial x}\right)x,e_j\right)+(B_{q-2}f)(|x|)\tau(\calB_\lambda(x|e_j),e_j)\right]}\\
 \stackrel{\eqref{eq:ddxradial}}{=}{}& 2(B_{q-2}^2f)(|x|)|x'|^2+\frac{2}{|x|}(B_{q-2}f)'(|x|)\sum_{j=1}^p{\tau\left(P\left(\left.\alpha x\right|\alpha e_j\right)x,e_j\right)}+\frac{d}{2}(B_{q-2}f)(|x|)\sum_{j=1}^p{(e_j|e_j)}\\
 ={}& (B_{q-2}^2f)(|x|)|x|^2+\frac{2}{|x|}(B_{q-2}f)'(|x|)\sum_{j=1}^p{\tau\left(P\left(\left.\alpha x\right|\alpha e_j\right)x,e_j\right)}+pd(B_{q-2}f)(|x|)
\end{align*}
and similarly for $\sum_{j=p+1}^n{\td\pi(e_j,0,-\alpha e_j)^2\psi(x)}$. Now a direct computation shows that
\begin{align*}
 \tau(P(\alpha x,\alpha e_j)x,e_j) &= |x|^2 & \forall j=1,\ldots,n.
\end{align*}
Therefore we obtain
\begin{multline*}
 -\sum_{j=1}^n{\td\pi(e_j,0,-\alpha e_j)^2\psi(x)}\\
 = |x|^2(B_{q-2}^2f)(|x|)+2p|x|(B_{q-2}f)'(|x|)+dp(B_{q-2}f)(|x|)\\
 + |x|^2(B_{p-2}^2f)(|x|)+2q|x|(B_{p-2}f)'(|x|)+dq(B_{p-2}f)(|x|)
\end{multline*}
which turns out to be equal to $2D_{\mu,\nu}+(q-p)(p+q-2)$. Taking into account that $(\frac{1}{\sqrt{2}}e_j)_j$ forms an orthonormal basis of $V$ with respect to $(-|-)$ we obtain
\begin{align*}
 \td\pi(C)\psi(x) &= \frac{r}{8n}\sum_{j=1}^n{\td\pi\left(\frac{1}{\sqrt{2}}e_j,0,-\frac{1}{\sqrt{2}}\alpha e_j\right)^2\psi(x)}\\
 &= -\frac{r}{8n}\left(D_{\mu,\nu}+\frac{(q-p)(p+q-2)}{2}\right)
\end{align*}
which finishes the proof of Theorem \ref{thm:CasimirAction}.

\chapter{Parabolic subgroups}\label{app:Parabolics}

Let $G$ be a real reductive group of inner type (i.e. $\Ad(G)\subseteq\Int(\frakg_\CC)$) and $\frakg=\frakk+\frakp$ be a Cartan decomposition of its Lie algebra. Further, let $P=MAN$ be any parabolic subgroup of $G$, not necessarily minimal. In this section we provide a construction of all standard parabolic subgroups containing $P$, only in terms of root data with respect to the abelian part $\fraka=\Lie(A)\subseteq\frakp$ of $P$. Note that $\fraka\subseteq\frakp$ is not necessarily maximal abelian.

For $\alpha\in\fraka^*$ we consider the weight space
\begin{align*}
 \frakg_\alpha := \{X\in\frakg:[H,X]=\alpha(H)X\ \forall H\in\fraka\}.
\end{align*}
Denote by $\Sigma(\frakg,\fraka)$ the root system of all $0\neq\alpha\in\fraka^*$ such that $\frakg_\alpha\neq0$. Choose a positive system $\Sigma^+(\frakg,\fraka)\subseteq\Sigma(\frakg,\fraka)$ and denote by $\Pi(\frakg,\fraka)$ the corresponding set of simple roots. For any finite subset $F\subseteq\Pi(\frakg,\fraka)$ of simple roots we form the Lie algebras
\begin{align*}
 \fraka_F &:= \{H\in\fraka:\alpha(H)=0\ \forall\alpha\in F\} \subseteq \fraka,\\
 \frakm_F &:= \{X\in\frakg:[X,\fraka_F]=0\}
\intertext{with corresponding Lie groups}
 A_F &:= \exp(\fraka_F),\\
 M_F &:= \{g\in G:\Ad(g)H=H\ \forall H\in\fraka_F\}.
\end{align*}
Further put
\begin{align*}
 \Sigma_F^+(\frakg,\fraka) &:= \{\alpha\in\Sigma^+(\frakg,\fraka):\alpha|_{\fraka_F}\neq0\}
\intertext{and}
 \frakn_F &:= \bigoplus_{\alpha\in\Sigma_F^+(\frakg,\fraka)}{\frakg_\alpha},\\
 N_F &:= \exp(\frakn_F).
\end{align*}
Finally we define
\begin{align*}
 P_F &:= M_FN_F.
\end{align*}

\begin{theorem}
\begin{enumerate}
\item[\textup{(1)}] The map
\begin{align*}
 \left\{\begin{array}{c}\mbox{finite subsets}\\\mbox{of $\Pi(\frakg,\fraka)$}\end{array}\right\} &\rightarrow \left\{\begin{array}{c}\mbox{standard parabolic subgroups}\\\mbox{of $G$ containing $P$}\end{array}\right\},\\
 F &\mapsto P_F,
\end{align*}
is a bijection.
\item[\textup{(2)}] Each $P_F$ has the Langlands decomposition $P_F=^\circ\!\! M_FA_FN_F$, where
\begin{align*}
 ^\circ\! M_F &= \{g\in M_F:\chi(g)=1\ \forall\mbox{characters }\chi:M_F\rightarrow\RR_+\},
\end{align*}
and the maps
\begin{align*}
 M_F\times N_F &\rightarrow P_F, & (m,n) &\mapsto mn,\\
 ^\circ\! M_F\times A_F\times N_F &\rightarrow P_F, & (m,a,n) &\mapsto man,
\end{align*}
are diffeomorphisms.
\item[\textup{(2)}] $G=KP_F$ and we have the following integral formula for $f\in C_c(G)$:
\begin{align*}
 \int_G{f(g)\td g} &= \int_K{\int_{^\circ\! M_F}{\int_{A_F}{\int_{N_F}{f(kman)a^{-2\rho_F}\td n}\td a}\td m}\td k},
\end{align*}
where $\td g$, $\td k$, $\td m$, $\td a$ and $\td n$ denote suitably normalized Haar measures on $G$, $K$, $^\circ\! M_F$, $A_F$ and $N_F$, respectively, and
\begin{align*}
 \rho_F(H) &= \frac{1}{2}\Tr(\ad(H)|_{\frakn_F}) = \frac{1}{2}\sum_{\alpha\in\Sigma_F^+(\frakg,\fraka)}{\dim(\frakg_\alpha)\cdot\alpha}
\end{align*} 
is the half sum of positive roots in $\Sigma_F^+(\frakg,\fraka)$.
\end{enumerate}
\end{theorem}

\begin{proof}
Choose a maximal abelian subalgebra $\widetilde{\fraka}$ of $\frakp$ that contains $\fraka$: $\fraka\subseteq\widetilde{\fraka}\subseteq\frakp$. We denote the weight space with respect to $\alpha\in\widetilde{\fraka}^*$ by $\widetilde{\frakg}_\alpha$. Then clearly
\begin{align*}
 \widetilde{\frakg}_\alpha &\subseteq \frakg_{\widehat{\alpha}},
\end{align*}
where $\widehat{\alpha}=\alpha|_{\fraka}$. Since $\frakg=\bigoplus_{\alpha\in\fraka^*}{\frakg_\alpha}=\bigoplus_{\alpha\in\widetilde{\fraka}^*}{\widetilde{\frakg}_\alpha}$, we conclude that
\begin{align*}
 \Phi:\Sigma(\frakg,\widetilde{\fraka})\cup\{0\} &\rightarrow \Sigma(\frakg,\fraka)\cup\{0\}, \alpha\mapsto\widehat{\alpha}=\alpha|_\fraka,
\end{align*}
is defined and surjective. One can choose a positive system $\Sigma^+(\frakg,\widetilde{\fraka})$ of $\Sigma(\frakg,\widetilde{\fraka})$ with corresponding simple roots $\Pi(\frakg,\widetilde{\fraka})$ such that $\Phi$ restricts to surjections
\begin{align*}
 \Phi^+:\Sigma^+(\frakg,\widetilde{\fraka})\cup\{0\}&\rightarrow\Sigma^+(\frakg,\fraka)\cup\{0\}, &&\mbox{and}& \Phi_\Pi:\Pi(\frakg,\widetilde{\fraka})\cup\{0\}&\rightarrow\Pi(\frakg,\fraka)\cup\{0\}.
\end{align*}
Then put $\widetilde{F}:=\Phi_\Pi^{-1}(F)\cup(\Pi(\frakg,\widetilde{\fraka})\setminus\Phi_\Pi^{-1}(\Pi(\frakg,\fraka)))\subseteq\Pi(\frakg,\widetilde{\fraka})$. The statements now follow immediately from \cite[Lemmas 2.2.7, 2.2.8 and 2.4.1]{Wal88} applied to $\widetilde{F}$.
\end{proof}

\chapter{Special Functions}\label{app:SpecialFunctions}

In this section we give definitions and basic properties of the special functions that appear in this paper.

\section{Bessel functions}

The series
\begin{align*}
 I_\alpha(z) &:= \left(\frac{z}{2}\right)^\alpha\sum_{n=0}^\infty{\frac{1}{j!\Gamma(j+\alpha+1)}\left(\frac{z}{2}\right)^n}
\end{align*}
defines a meromorphic function in $z$ and $\alpha$ called the modified Bessel function of the first kind or $I$-Bessel function (see \cite[Section 3.7]{Wat44}). For $\alpha\in\RR$ and $z>0$ this function takes real values. $I_\alpha(z)$ solves the following second order differential equation:
\begin{align}
 z^2\frac{\td^2u}{\td z^2}+z\frac{\td u}{\td z}-(z^2+\alpha^2)u &= 0.\label{eq:DiffEqBessel}
\end{align}
Another solution of \eqref{eq:DiffEqBessel} which is linearly independent of $I_\alpha(z)$ is given by the modified Bessel function of third kind or $K$-Bessel function:
\begin{align*}
 K_\alpha(z) &:= \frac{\pi}{2\sin\pi\alpha}(I_{-\alpha}(z)-I_\alpha(z)).
\end{align*}
For convenience we use the following renormalizations:
\begin{align*}
 \widetilde{I}_\alpha(z) &:= \left(\frac{z}{2}\right)^{-\alpha}I_\alpha(z), & \widetilde{K}_\alpha(z) &:= \left(\frac{z}{2}\right)^{-\alpha}K_\alpha(z).
\end{align*}
E.g. for $\alpha=-\frac{1}{2}$ we obtain
\begin{align*}
 \widetilde{I}_{-\frac{1}{2}}(z) &= \frac{1}{\sqrt{\pi}}\cosh(z), & \widetilde{K}_{-\frac{1}{2}}(z) &= \frac{\sqrt{\pi}}{2}e^{-z}.
\end{align*}
Corresponding to \eqref{eq:DiffEqBessel}, $\widetilde{I}_\alpha(z)$ and $\widetilde{K}_\alpha(z)$ solve the second order equation
\begin{align}
 z^2\frac{\td^2u}{\td z^2}+(2\alpha+1)z\frac{\td u}{\td z}-z^2u &= 0,\label{eq:DiffEqModBessel}
\end{align}
or equivalently
\begin{align}
 \left(\theta^2+2\alpha\theta-z^2\right)u &= 0,\label{eq:DiffEqModBesselTheta}
\end{align}
where $\theta=z\frac{\td}{\td z}$. For the normalized $K$-Bessel function one has the differential recurrence relation (see \cite[Equation 3.71 (6)]{Wat44})
\begin{align}
 \frac{1}{z}\widetilde{K}_\alpha'(z) &= -\frac{1}{2}\widetilde{K}_{\alpha+1}(z),\label{eq:KBesselDiffRecRel}
\end{align}
with which the differential equation \eqref{eq:DiffEqModBessel} can equivalently be written as a recurrence relation:
\begin{align}
 \alpha\widetilde{K}_\alpha(z) &= \left(\frac{z}{2}\right)^2\widetilde{K}_{\alpha+1}(z)-\widetilde{K}_{\alpha-1}(z).\label{eq:KBesselRecRel}
\end{align}
Restricted to the positive real line $\RR_+$ the normalized $K$-Bessel function has the following asymptotic behaviour (see \cite[Chapters III and VII]{Wat44} and \cite[Chapter 4]{AAR99}):
\begin{align}
 \widetilde{K}_\alpha(x) &= \left\{\begin{array}{ll}\frac{\Gamma(\alpha)}{2}\left(\frac{x}{2}\right)^{-2\alpha}+o(x^{-2\alpha}) &\mbox{if $\alpha>0$,}\\-\log(\frac{x}{2})+o(\log(\frac{x}{2})) &\mbox{if $\alpha=0$,}\\\frac{\Gamma(-\alpha)}{2}+o(1) &\mbox{if $\alpha<0$,}\end{array}\right. & \mbox{as }x &\rightarrow 0,\label{eq:KBesselAsymptAt0}\\
 \widetilde{K}_\alpha(x) &= \frac{\sqrt{\pi}}{2}\left(\frac{x}{2}\right)^{-\alpha-\frac{1}{2}}e^{-x}\left(1+\mathcal{O}\left(\frac{1}{x}\right)\right), & \mbox{as }x &\rightarrow\infty.\label{eq:BesselAsymptAtInfty}
\end{align}

\section{Meijer's $G$-function}

The $G$-function can be defined in a very general setting. However, we restrict our definition to the case which is needed in this paper. The results in this section are taken from \cite[Chapter V]{Luk69}.

Let $0\leq m\leq q$, $0\leq n\leq p$, $p<q$ and $a_1,\ldots,a_p,b_1,\ldots,b_q\in\CC$. Assume further that $a_k-b_j$ is not a positive integer for $j=1,\ldots,m$, $k=1,\ldots,n$. For $z\neq0$ in the univeral covering of $\CC^\times$ we define
\begin{align*}
 G^{m,n}_{p,q}\left(z\left|\begin{array}{cc}a_1,\ldots,a_p\\b_1,\ldots,b_q\end{array}\right.\right) &:= \frac{1}{2\pi i}\int_L{\frac{\prod_{j=1}^m{\Gamma(b_j-s)}\prod_{j=1}^n{\Gamma(1-a_j+s)}}{\prod_{j=m+1}^q{\Gamma(1-b_j+s)}\prod_{j=n+1}^p{\Gamma(a_j-s)}}z^s\td s}.
\end{align*}
Here $L$ is a loop beginning and ending at $+\infty$ and encircling all poles of $\Gamma(b_j-s)$, $j=1,\ldots,m$, once in the negative direction, but none of the poles of $\Gamma(1-a_k+s)$, $k=1,\ldots,n$. $G^{m,n}_{p,q}(z|^{a_p}_{b_q})$ is called \textit{Meijer's $G$-function}. From the definition one immediately obtains the reduction formula (cf. \cite[Equation 5.4 (1)]{Luk69})
\begin{align}
 G^{m,n}_{p,q}\left(z\left|\begin{array}{cc}a_1,\ldots,a_p\\b_1,\ldots,b_{q-1},a_1\end{array}\right.\right) &= G^{m,n-1}_{p-1,q-1}\left(z\left|\begin{array}{cc}a_2,\ldots,a_p\\b_1,\ldots,b_{q-1}\end{array}\right.\right).\label{eq:GFctRed}
\end{align}
The $G$-function $G^{m,n}_{p,q}(z|^{a_p}_{b_q})$ solves the following differential equation of order $\max(p,q)$ (see \cite[Equation 5.8 (1)]{Luk69}):
\begin{align}
 \left[(-1)^{m+n-p}z\prod_{j=1}^p{(\theta-a_j+1)}-\prod_{k=1}^q{(\theta-b_k)}\right]u &= 0,\label{eq:GFctDiffEq}
\end{align}
where $\theta=z\frac{\td}{\td z}$. Further, the $J$- and $K$-Bessel functions can be expressed in terms of $G$-functions (see \cite[Equations 6.4 (8) \& (11)]{Luk69})
\begin{align}
 \left(\frac{z}{4}\right)^\beta J_\alpha(z) &= G^{20}_{04}\left(\left.\left(\frac{z}{4}\right)^4\right|\frac{\beta+\alpha}{4},\frac{\beta+\alpha+2}{4},\frac{\beta-\alpha}{4},\frac{\beta-\alpha+2}{4}\right),\label{eq:GFctJBessel}\\
 2\left(\frac{z}{2}\right)^\beta K_\alpha(z) &= G^{20}_{02}\left(\left.\left(\frac{z}{2}\right)^2\right|\frac{\beta+\alpha}{2},\frac{\beta-\alpha}{2}\right).\label{eq:GFctKBessel}
\end{align}
We also need the following integral formula for the $G$-function $G^{20}_{04}(z|b_1,b_2,b_3,b_4)$ which holds for $\omega,\eta>0$ and $\Re(b_j-a\pm\frac{\alpha}{2})>-1$ ($j=1,2$) (see \cite[Equation 5.6 (21), assumptions as in case 4]{Luk69}):
\begin{multline}
 \int_0^\infty{x^{-a}K_\alpha(2(\omega x)^{\frac{1}{2}}))G^{20}_{04}(\eta x|b_1,b_2,b_3,b_4)\td x}\\
 = \frac{\omega^{a-1}}{2}G^{22}_{24}\left(\frac{\eta}{\omega}\left|\begin{array}{c}a+\frac{\alpha}{2},a-\frac{\alpha}{2}\\b_1,b_2,b_3,b_4\end{array}\right.\right).\label{eq:GFctIntKBessel}
\end{multline}
Finally we give the asymptotic behaviour of the function $G^{20}_{04}(z|b_1,b_2,b_3,b_4)$ as $z\rightarrow0$ and $z\rightarrow\infty$. For the asymptotics as $z\rightarrow0$ we assume without loss of generality that $b_1\leq b_2$. Then it follows from \cite[Equations 5.2 (7) \& (10)]{Luk69} that
\begin{multline}
 G^{20}_{04}(z|b_1,b_2,b_3,b_4)\\
 = \frac{1}{\Gamma(1+b_1-b_3)\Gamma(1+b_1-b_4)}\times\begin{cases}\Gamma(b_2-b_1)z^{b_1}+o(z^{b_1}) & \mbox{if }b_1<b_2,\\-\ln(z)z^{b_1}+o(\ln(z)z^{b_1}) & \mbox{if }b_1=b_2.\end{cases}\label{eq:GFctAsymptotics0}
\end{multline}
For the asymptotic behaviour as $x\rightarrow\infty$ (on the real line) we find with \cite[Section 5.10, Theorem 2]{Luk69} that
\begin{align}
 G^{20}_{04}(x|b_1,b_2,b_3,b_4) = -\frac{1}{\sqrt{2\pi}}x^\theta\cos\left(4x^{\frac{1}{4}}+(b_3+b_4-2\theta)\pi\right)\left(1+\calO(x^{-\frac{1}{4}})\right),\label{eq:GFctAsymptoticsInfty}
\end{align}
where $\theta=\frac{1}{4}(b_1+b_2+b_3+b_4-\frac{3}{2})$.

\section{The functions $\Lambda_j^{\mu,\nu}(x)$}

Yet to be written

\chapter{The metaplectic representation}

Let $V=\Sym(n,\RR)$. Then $L=\Str(V)_0=\RR_+\SL(n,\RR)$ and hence $\frakl=\frakg\frakl(n,\RR)$. The map
\begin{align*}
 \frakg \rightarrow \sp(n,\RR),\ (u,T,v)\mapsto\left(\begin{array}{cc}T&u\\v&-T^t\end{array}\right),
\end{align*}
is an isomorphism of Lie algebras. The elements $c_i:=E_{ii}$, $i=1,\ldots,n$, form a Jordan frame. The orbit $\calO$ is given by
\begin{align*}
 \calO &= \{g\cdot c_1=gc_1g^t:g\in L\} = \{xx^t:x\in\RR^n,x\neq0\}.
\end{align*}
Further, the map
\begin{align*}
 \RR^n\setminus\{0\}\rightarrow\calO_1,\ x\mapsto xx^t,
\end{align*}
induces an isomorphism of the $L^2$-spaces
\begin{align*}
 \calU:L^2(\calO_1,\td\mu_1)\rightarrow L^2_{\textup{even}}(\RR^n),\ \calU\psi(x) := \psi(xx^t).
\end{align*}
Isometry can be seen as follows:
\begin{align*}
 \int_{\RR^n}{|\calU\psi(x)|^2\td x} &= \int_{\SO(n)}{\int_0^\infty{|\calU\psi(kte_1)|^2t^{n-1}\td t}\td k}\\
 &= \int_{\SO(n)}{\int_0^\infty{|\psi(t^2kc_1k^t)|^2t^{n-1}\td t}\td k}\\
 &= \frac{1}{2}\int_{\SO(n)}{\int_0^\infty{|\psi(k\cdot sc_1)|^2s^{\frac{n}{2}-1}\td s}\td k}\\
 &= \frac{1}{2}\int_\calO{|\psi(x)|^2\td\mu(x)}.
\end{align*}
Conjugating the representation $\pi$ of $G=G_0=\PP\Sp(n,\RR)$ with $\calU$ defines a representation $\widetilde{\pi}$ of $\Sp(n,\RR)$ on $L^2_{\textup{even}}(\RR^n)$. \textcolor{red}{We will show that $\widetilde{\pi}$ is the metaplectic representation as studied in \cite{Fol89}.}
